# Supplementary material for: Energy-Based Models for Continual Learning
Source: arXiv:2011.12216 source file (2022-12-18)
Supplement: Supplementary file 1 [file fisher.tex]

\begin{figure*}[h]
\begin{center}
\includegraphics[width=0.8\linewidth]{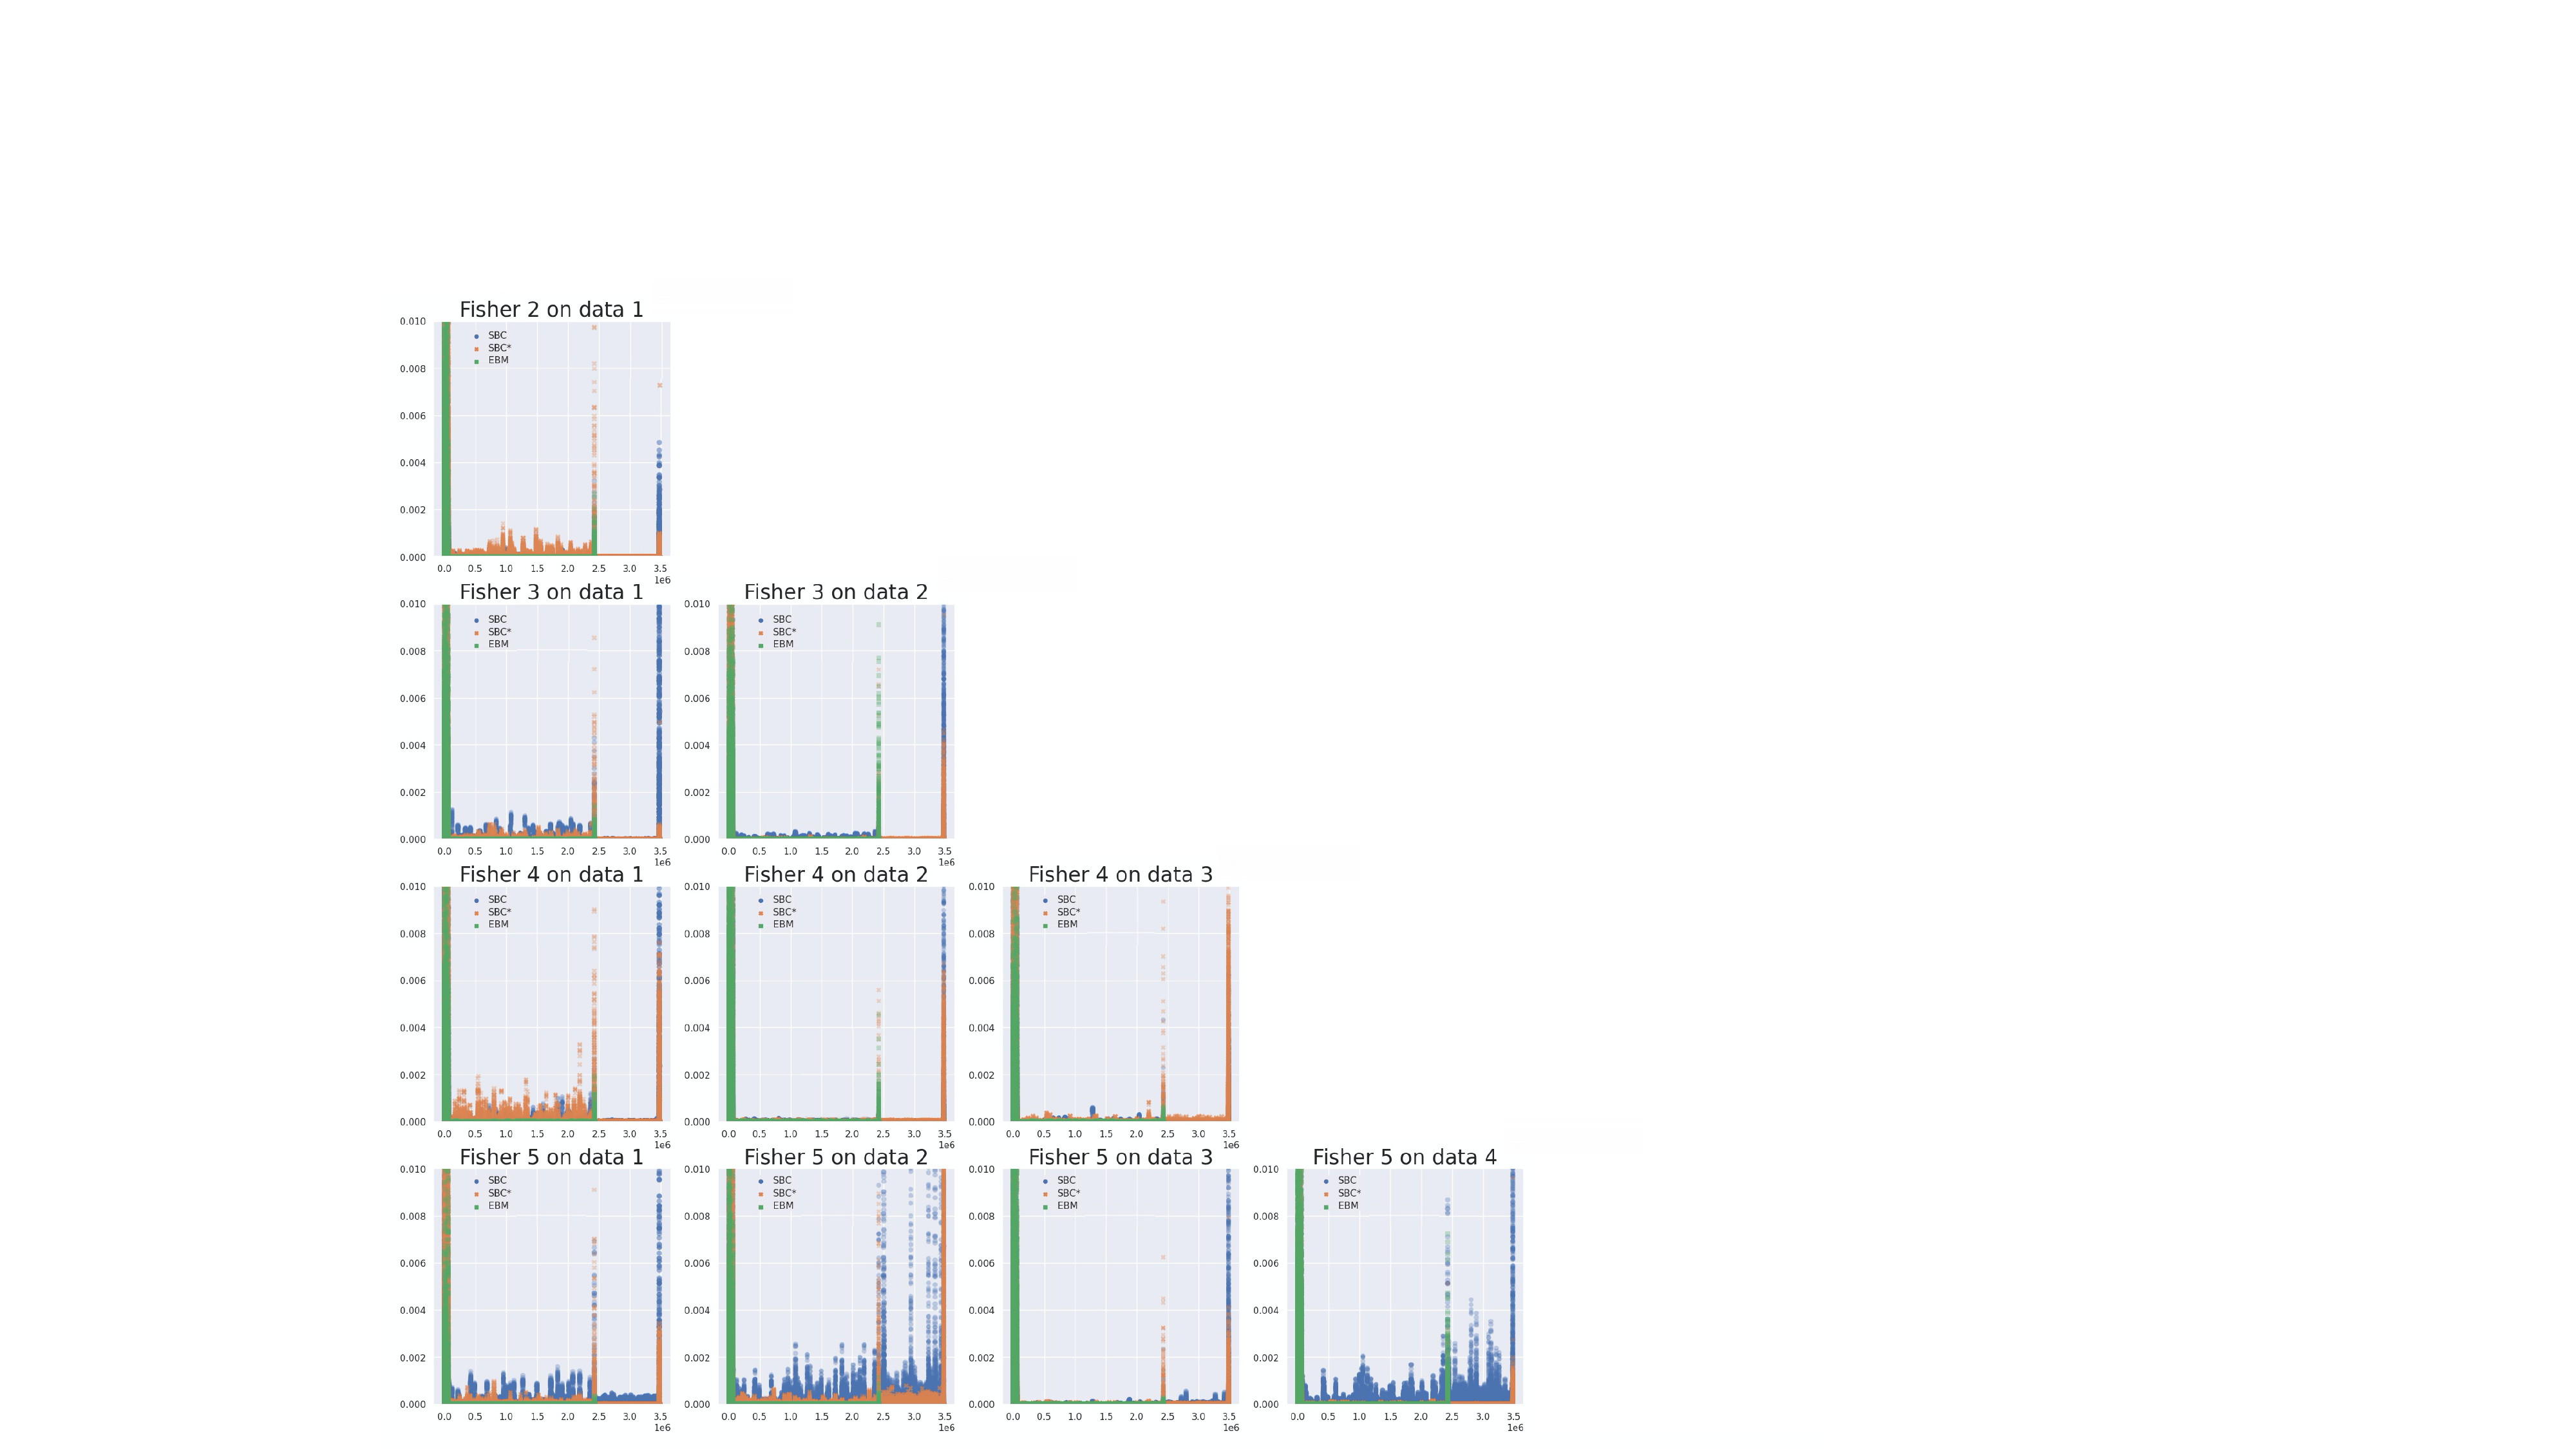}
\end{center}
\vspace{-5pt}
\caption{\small{Parameter importance on different tasks. The x-axis represents each different parameter and y-axis is the FIM value in \eqn{eqn:fisher}. The sparser the parameters are, the fewer important parameters there are for previous data. The sparsity of parameter importance in EBMs may explain why EBMs have less influence on previous tasks after training on new data.
% train on the new data has less influence on previous tasks.
% the better the model is in learning new tasks with less influence on previous tasks. 
``Fisher 5 on data 1'' means the diagonal elements of the fisher information matrix obtained by \eqn{eqn:fisher} using the model parameters $\theta_5$ (after training on task $T_5$) and data from task $T_1$.}}
\vspace{-5pt}
\label{fig:fisher}
\end{figure*}
