# Supplementary material for: Energy-Based Models for Continual Learning
Source: arXiv:2011.12216 source file (2022-12-18)
Supplement: Supplementary file 2 [file training_curve.tex]

\begin{figure*}[h]
\begin{center}
\includegraphics[width=1\linewidth]{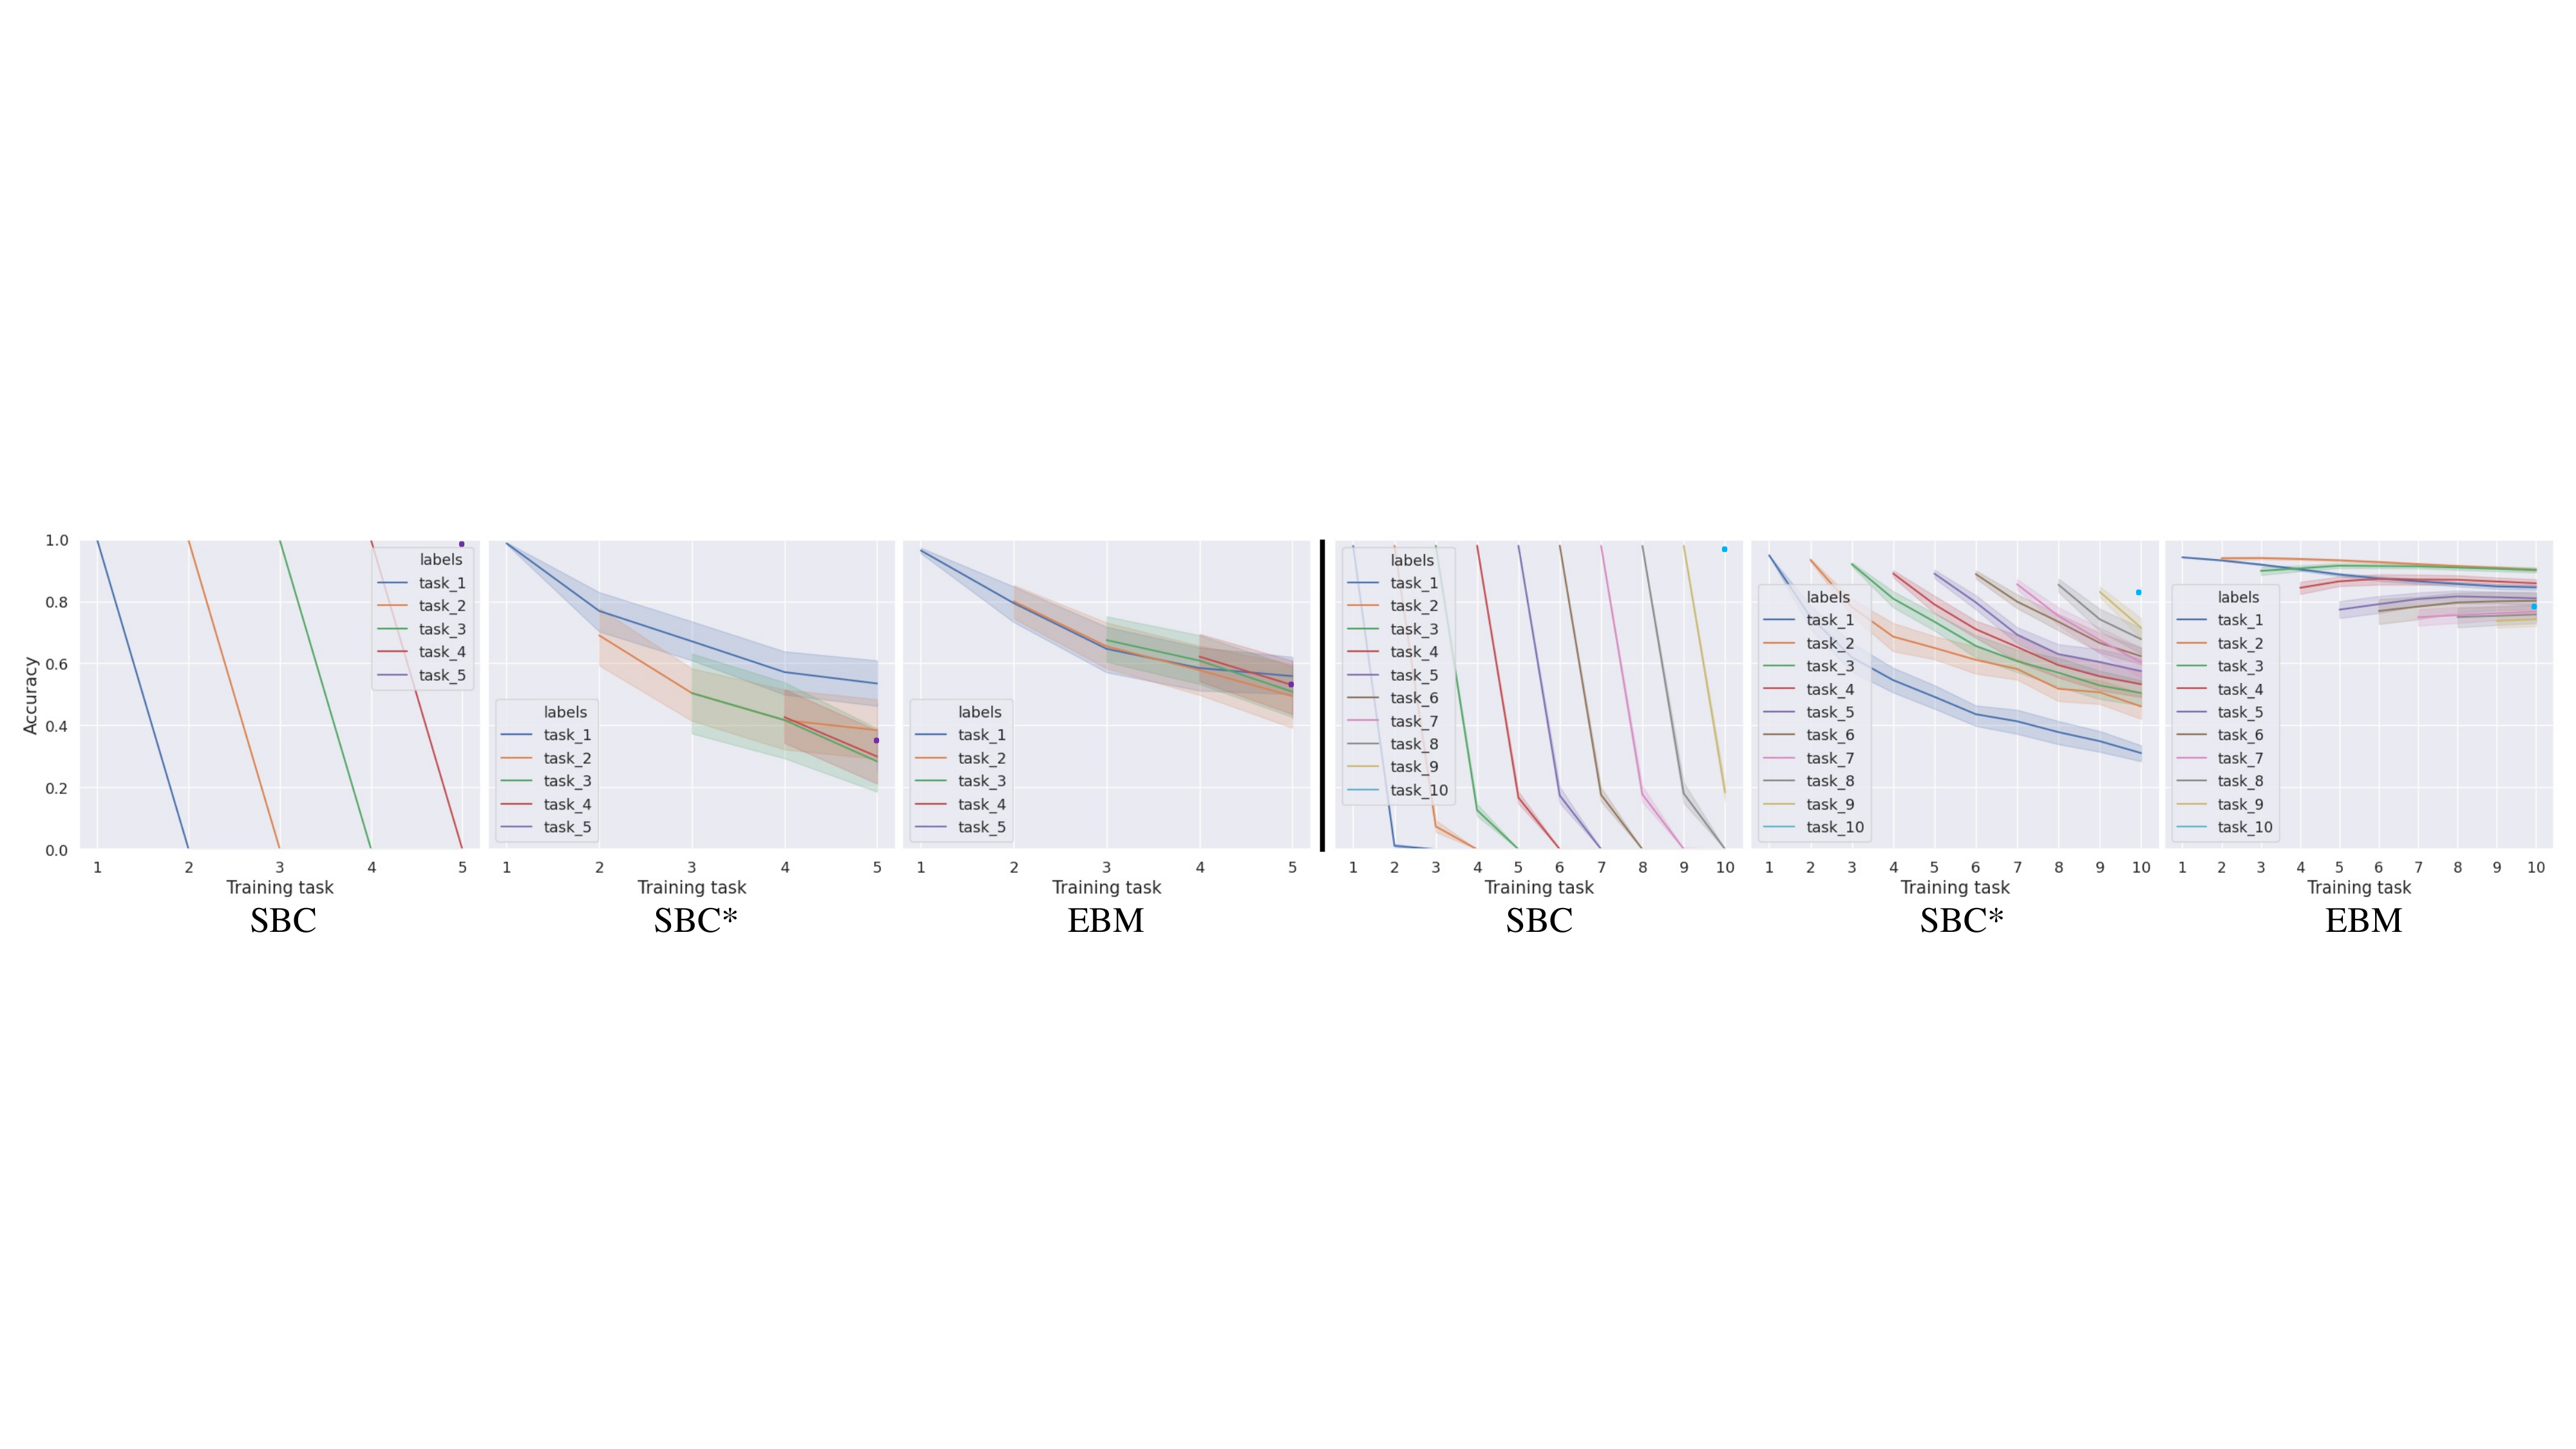}
\end{center}
\vspace{-5pt}
\caption{\small{\emph{Class-IL} testing accuracy of the standard classifier (SBC), classifier using our training objective (SBC*), and EBMs on each task on the split MNIST dataset (left) and permuted MNIST dataset (right).}}
\label{fig:training_curve}
\end{figure*}
